# Supplementary material for: Latent Variable Representation for Reinforcement Learning
Source: arXiv:2212.08765 source file (2023-03-07)
Supplement: Supplementary file 1 [file appendix.tex]

\paragraph{Transition decomposition}
\Tongzheng{Check this part later.}
We decompose the transition probability using a latent variable $z$ such that
\begin{align}
P(s'|s, a) & = \int P(s^\prime|z) P(z|s, a)dz 
\\
& = 
\int_z \int_{x}\ker (z, x) \alpha_{s'} (x) P(x) d x P(z|s,a) dz
\\
& = 
\int_z \int_{x} \left\langle \phi(x), \phi(z) \right\rangle \alpha_{s'} (x) P(x) d x P(z|s,a) dz
\\
& =
\left\langle \int_z \phi(z) P(z|s,a)dz,  \int_{z}   \alpha_{s'} (z) \phi(z) P(z) dz \right\rangle 
\\
& = 
\left\langle \phi(s,a),  \mu(s') \right\rangle \, .
\end{align}
where we use $\ker(z,x) = \left\langle \phi(z), \phi(x) \right\rangle$ and write $\phi(s,a) =  \int_z \phi(z) P(z|s,a) dz$. 
Since we have a linear MDP now, 
the q-function can be written as
\begin{align}
q(s,a) 
& = \int_z \int_{x}\ker (z, x) \alpha (x) P(x) d x P(z|s,a) dz
\\
& = \int_{x} \alpha(x) P(x) \int_z P(z|s,a) \ker(x, z) dz dx
\\
%& \approx \int_{x} \alpha(x) P(x) \left\langle \phi(x), \frac{1}{n} \sum_{j=1}^n \phi(f_\theta(s,a,\epsilon_i )) \right\rangle dx \\
& \approx 
\frac{1}{n} \sum_{i=1}^n \alpha(x_i) \ker(x_i, f_\theta(s,a,\epsilon_i))
\end{align}
where $\alpha(z) = \int_s \alpha_s(z) ds$.
